# Supplementary material for: SMART: Scalable Multi-agent Real-time Motion Generation via Next-token Prediction
Source: arXiv:2405.15677 source file (2024-11-01)
Supplement: Supplementary file 1 [file appendix.tex]

%%%%%%%%%%%%%%%%%%%%%%%%%%%%%%%%%%%%%%%%%%%%%%%%%%%%%%%%%%%%
\newpage

\newpage
